# Supplementary material for: Hgformer: Hyperbolic Graph Transformer for Recommendation
Source: arXiv:2502.15693 source file (2024-12-30)
Supplement: Supplementary file 1 [file appendix.tex]

\newpage
\appendix

\section{Notations}
\label{notations}
All the notations and their descriptions used in this paper are summarized in Table~\ref{rec-notation}.

\setlength{\textfloatsep}{0.1cm}
\begin{table}[H]
	\centering
	\caption{{{Notations used in this paper}}}
	\vspace{-0.cm}
	
	\scalebox{0.85}{
		\begin{threeparttable} 
			\begin{tabular}{p{2.5cm}<{\centering}|p{5.4cm}<{\centering}}
				\hline\hline
				Notation  & Description \\ \hline
$\mathcal{V}_u$ \& $\mathcal{V}_i$  &The user and item set\\ 
$N$  &Number of users \\   
$M$  &Number of items\\
$N_i$ & The neighbors of node i\\
$\mathcal{E}$ &Interactions between users and items\\
$\Theta$ &Model parameters\\
$d$  &Dimension of latent embeddings.\\  
$\textbf{u}^{\mathcal{E}}$ \& $\textbf{i}^{\mathcal{E}}$ &User\&item embeddings in Euclidean space.\\
$\textbf{u}$ \& $\textbf{i}$ & User\&item embeddings in hyperbolic manifold.\\
$\textbf{u}_k$ \& $\textbf{i}_l$ & $k$-th and $l$-th vector of $\textbf{u}$ \& $\textbf{i}$ \\
$\textbf{u}^{(l)}$ \& $\textbf{i}^{(l)}$ & User\&item embeddings after $l$-th layer of LHGCN\\
$\textbf{q}_i^{(h)}$ \& $\textbf{k}_j^{(h)}$\& $\textbf{v}_j^{(h)}$ & $i$-th query, $j$-th key and value of $h$-head\\%The queries of $i$-th user and keys of $j$-th item values keys of $k$-th item. The hyper script $h$ means $h$-th head of the self-attention mechanism\\
$\mathbf{u}^{local}$ \& $\mathbf{i}^{local}$ & User\&item embeddings after LHGCN\\
$\mathbf{u}^{global}$ \& $\mathbf{i}^{global}$ & User\&item embeddings of hyperbolic cross attention.\\ 
$w_{i,j}^{(h)}$ & Similarity score of $i$-th user and $j$-item of $h$-th head in the self-attention\\
$\hat{\mathbf{u}}_i^{(h)}$ & $i$-th user embedding of $h$-th head after Euclidean weighted sum.\\
$\mathbf{u}_i'^{(h)}$ & $i$-th user embedding of $h$-th head after hyperbolic weighted sum.\\
$m$ & Number of random features.\\
%$\tau$ & A hyperparameter, temperature.\\
%$-1/K$ & A hyperparameter, curvature of a hyperbolic manifold.\\
%$\alpha$ & A hyperparameter, between 0 and 1.\\
%$m$ & Number of features in kernel function.\\
%\lambda$ & Is a non-negative hyperparameter.\\
                    
                    \hline
				\hline
			\end{tabular}
	\end{threeparttable} }
	\label{rec-notation}
	\vspace{-0.cm}
\end{table}

\section{Proof of Theorem 4.1}
\label{pft1}
\input{proofs/theorem1proof}

\section{Proof of Lemma 4.2}
\label{pfl}
\input{proofs/lemma2proof}
\section{Proof of Theorem 4.2}
\label{pft2}
\input{proofs/theorem2proof}

%\cite{rendle2012bpr,xue2017deep,zheng2018spectral,wang2019neural,lightgcn}
\section{Details of baseline models}
\label{setting}
%补上几个CF的算法和几个图算法做对比
\subsection{Description of baseline models} We introduce the baseline models in detail as follows:
\begin{itemize}
\item[$\bullet$] \textbf{BPR} \cite{rendle2012bpr}is a basic matrix factorization model that is trained in a pairwise way.
\item[$\bullet$] \textbf{DMF} \cite{xue2017deep}is a neural network enhanced matrix factorization model.
% \item[$\bullet$] \textbf{MultiVAE} \cite{liang2018variational}is an item-based collaborative filtering model that simultaneously ranks all items for each user.
% \item[$\bullet$] \textbf{SpectralCF} \cite{zheng2018spectral}is a spectral convolution model that directly learns latent factors of users and items from the spectral domain for recommendation.
% \item[$\bullet$] \textbf{NGCF} \cite{wang2019neural}is a model that incorporate GNN for recommendation.
\item[$\bullet$] \textbf{LightGCN} \cite{lightgcn} is a classic graph-based method that leverages linear GNNs for recommendation.
\item[$\bullet$] \textbf{HMLET} \cite{kong2022linear} combines both linear and non-linear propagation layers for general recommendation and yields better performance.
\item[$\bullet$] \textbf{HGCF} \cite{hgcf} is a hyperbolic graph neural network model for recommendation. 

\item[$\bullet$] \textbf{HRCF} \cite{hrcf} is a hyperbolic graph neural network model with geometric regularization for recommendation.
\item[$\bullet$] \textbf{HICF} \cite{hicf} is a hyperbolic graph neural network model with geometric aware margin ranking learning for recommendation.
% \item[$\bullet$] \textbf{GFormer} \cite{gformer} is the state-of-the-art method that automates the self-supervision augmentation with transformer architecture.
\item[$\bullet$] \textbf{SGFormer} \cite{sgformer} a linear graph transformer model for scalable graphs.
\item[$\bullet$] \textbf{NodeFormer} \cite{nodeformer} a kernel function-based graph transformer model for scalable graphs.
\end{itemize}

\subsection{Implementations of proposed model}
\label{app:imple}
For BPR, DMF, and SpectralCF we adopted the implementation of RecBole, and for LightGCN and HMLET we adopted the implementation of RecBole-GNN.\footnote{\url{https://github.com/RUCAIBox/RecBole-GNN/}} For HGCF, HICF, HRCF, SGFormer, and NodeFormer, we integrated their source code into the RecBole-GNN framework based on their original implementations.\footnote{\url{https://github.com/layer6ai-labs/HGCF}} \footnote{\url{https://github.com/marlin-codes/HICF}} \footnote{\url{https://github.com/marlin-codes/HRCF}}
We used Adam as the optimizer for all models except HGCF, HICF, and HRCF, which are optimized using RSGD \cite{bonnabel2013stochastic}. For all the models, we tuned the learning rate from 2e-2 to 1e-5 and batch size from \([4096, 32768, 65536]\). The embedding size was set to 64. The layers of GNN-based models (LightGCN, HGCF, HRCF, HICF, Hgformer) were tuned from \([3, 4, 5, 6, 7, 8]\). The curvature of hyperbolic models was tuned from \([0.1, 0.5, 1.0]\).

\section{Formal definition of evaluation metrics}
\label{metrics}

% \section{Comparison of HGCF and LHGCN}
% The aggregation of LHGCN is given by 
% \begin{equation}
% \mathbf{Centroid}(\mathcal{N})= \sqrt{K}\frac{\sum_{\mathbf{x}_{i} \in \mathcal{N}}\mathbf{x}_{i}}{|\ \ ||\sum_{\mathbf{x}_{i}\in \mathcal{N}}\mathbf{x}_{i}||_\mathcal{M}|},
% \end{equation}
% which is a closed solution of the problem
% \begin{equation}
% \mathbf{Centroid}(\mathcal{N})=\arg\min _{\mathbf{c} \in \mathcal{H}^{d+1, K}} \sum_{{\mathbf{x}_{i}}\in \mathcal{N}}d_{\mathcal{M}}^K(\mathbf{c},\mathbf{x}_{i})^2.
% \end{equation}
% The proof is given in \cite{zhang2021lorentzian}. 
